# Supplementary material for: Continuous-Time Graph Learning for Cascade Popularity Prediction
Source: arXiv:2306.03756 source file (2023-06-06)
Supplement: Supplementary file 1 [file section-7-appendix.tex]

\appendix
\section{Appendix}

% \subsection{Baseline}
% \label{appendix:baseline}
% The extracted five types of feature in feature-based methods are edge number, max depth, average depth, breath of cascade graph, and publication time of the cascade. Casflow uses an additional node feature extracted from the social network built from observed data. To make a fair comparison, we do not use this additional node feature. For baseline implementation, if there is an official implementation, we use the official implementation, if not, we implement it ourselves.
